# Supplementary material for: Falcon 7b for Software Mention Detection in Scholarly Documents
Source: arXiv:2405.08514 source file (2024-05-14)
Supplement: Supplementary file 1 [file appendix.tex]

\section{Appendix}
\label{sec:app}

\begin{table}[h]
\centering
\caption{The hyperparameters used in training experiments.}
\begin{tabular}{ll}
\hline
\textbf{Hyperparameter}                & \textbf{Value}    \\ \hline
Number of Training Epochs              & 4                 \\
Learning Rate Scheduler Type           & Cosine            \\
Warmup Ratio                           & 0.03              \\
Maximum Gradient Norm                  & 0.3               \\
Learning Rate                          & 2e-4              \\
Use BF16 Precision                     & True              \\
Gradient Checkpointing                 & True              \\
Gradient Accumulation Steps            & 8                 \\
Per-device Training Batch Size         & 8                 \\
Per-device Evaluation Batch Size       & 8                 \\
Adam Beta1                             & 0.9               \\
Adam Beta2                             & 0.95              \\
Weight Decay                           & 0.0               \\
Evaluation Accumulation Steps          & 8                 \\
\hline
\end{tabular}
\label{table:hyperparameters}
\end{table}

\begin{table}[H]
\centering
\caption{Misclassification in software mention type: example 1.}
\begin{tabular}{l|l|l}
\textbf{Token}         & \textbf{Prediction}                & \textbf{Label}                     \\ \hline
At                     & O                                  & O                                  \\
present                & O                                  & O                                  \\
Chaste                 & O                                  & B-PlugIn\_Mention                  \\
can                    & O                                  & O                                  \\
only                   & O                                  & O                                  \\
be                     & O                                  & O                                  \\
used                   & O                                  & O                                  \\
with                   & O                                  & O                                  \\
Linux                  & B-OperatingSystem\_Usage           & B-OperatingSystem\_Mention         \\
,                      & O                                  & O                                  \\
although               & O                                  & O                                  \\
it                     & O                                  & O                                  \\
works                  & O                                  & O                                  \\
well                   & O                                  & O                                  \\
via                    & O                                  & O                                  \\
a                      & O                                  & O                                  \\
Linux                  & B-OperatingSystem\_Mention         & B-OperatingSystem\_Mention         \\
virtual                & O                                  & O                                  \\
machine                & O                                  & O                                  \\
(                      & O                                  & O                                  \\
using                  & O                                  & O                                  \\
software               & O                                  & O                                  \\
such                   & O                                  & O                                  \\
as                     & O                                  & O                                  \\
VirtualBox             & B-Application\_Mention             & B-Application\_Mention             \\
)                      & O                                  & O                                  \\
on                     & O                                  & O                                  \\
a                      & O                                  & O                                  \\
host                   & O                                  & O                                  \\
running                & O                                  & O                                  \\
Microsoft              & O                                  & O
                         \\
Windows                & B-OperatingSystem\_Usage           & B-OperatingSystem\_Mention \\
or                     & O                                  & O
                         \\
Mac                    & B-OperatingSystem\_Usage           & B-OperatingSystem\_Mention         \\
OS                     & I-OperatingSystem\_Usage           & I-OperatingSystem\_Mention         \\
X                      & I-OperatingSystem\_Usage                                   & I-OperatingSystem\_Mention                                  \\
.                      & O                                  & O                                  
\end{tabular}
\label{table:confusion_usage_mention}
\end{table}

\begin{table}[h]
\centering
\caption{Difficulty in multi-token classification}
\begin{tabular}{l|l|l}
\hline
\textbf{Input} & \textbf{Prediction} & \textbf{Label} \\
\hline
Here & O & O \\
, & O & O \\
we & O & O \\
present & O & O \\
a & O & O \\
new & O & O \\
web & O & O \\
server & O & O \\
- & O & O \\
based & O & O \\
tool & O & O \\
, & O & O \\
the & O & O \\
Pipeline & B-Application\_Creation & B-Application\_Creation \\
for & I-Application\_Creation & I-Application\_Creation \\
estimating & I-Application\_Creation & I-Application\_Creation \\
EPIStatic & I-PlugIn\_Creation & I-Application\_Creation \\
genetic & O & I-Application\_Creation \\
effects & O & I-Application\_Creation \\
( & O & O \\
PEPIS & O & O \\
) & O & O \\
, & O & O \\
for & O & O \\
analyzing & O & O \\
polygenic & O & O \\
epistatic & O & O \\
effects & O & O \\
. & O & O \\
\hline
\end{tabular}
\label{table:multi_token_misclassification}
\end{table}
